# Supplementary material for: Giant edge spin accumulation in a symmetric quantum well with two subbands
Source: arXiv:1602.00026 ancillary file (2017-02-13)
Supplement: Supplementary file 1 [file Supplemental_Material_2.pdf]

# Supplementary material for "Giant edge spin accumulation in a symmetric quantum well with two subbands"

Alexander Khaetskii[1] and J. Carlos Egues[2]

[1]*Department of Physics, University at Buffalo, SUNY, Buffalo, NY 14260-1500*

[2]*Instituto de Física de São Carlos, Universidade de São Paulo, 13560-970, São Carlos, São Paulo, Brazil*

## I. THE EIGENVECTORS OF HAMILTONIAN

For completeness here we present the explicit form or our Hamiltonian [Eq. (2) in the main text]. In the basis $\{|e\rangle_\uparrow, |o\rangle_\downarrow, |o\rangle_\uparrow, |e\rangle_\downarrow\}$ the Hamiltonian becomes [1]

$$H = \begin{pmatrix} \frac{p^2}{2m} + \varepsilon_e & -i\eta k_- & 0 & 0 \\ i\eta k_+ & \frac{p^2}{2m} + \varepsilon_0 & 0 & 0 \\ 0 & 0 & \frac{p^2}{2m} + \varepsilon_0 & -i\eta k_- \\ 0 & 0 & i\eta k_+ & \frac{p^2}{2m} + \varepsilon_e \end{pmatrix} \tag{S1}$$

Here $k_\pm = k_x \pm ik_y$, $m$ is the effective mass, $\varepsilon_e$ and $\varepsilon_o$ are the quantized energies of the lowest (even) and first excited (odd) subbands, respectively, measured from the bottom of the quantum well, $\eta$ is the inter-subband SO coupling. The kets $|i\rangle_\sigma$, $i = e, o$, $\sigma =\uparrow,\downarrow$ denote the corresponding two lowest eigestates. The Hamiltonian (S1) has the following 4 eigenstates

$$|\Psi_{1,\uparrow} >= e^{i\mathbf{kr}} \begin{pmatrix} \cos(\theta/2) \\ -ie^{i\varphi}\sin(\theta/2) \\ 0 \\ 0 \end{pmatrix}, \; |\Psi_{1,\downarrow} >= e^{i\mathbf{kr}} \begin{pmatrix} 0 \\ 0 \\ \sin(\theta/2) \\ -ie^{i\varphi}\cos(\theta/2) \end{pmatrix}, \tag{S2}$$

$$|\Psi_{2,\uparrow} >= e^{i\mathbf{kr}} \begin{pmatrix} 0 \\ 0 \\ \cos(\theta/2) \\ ie^{i\varphi}\sin(\theta/2) \end{pmatrix}, \; |\Psi_{2,\downarrow} >= e^{i\mathbf{kr}} \begin{pmatrix} \sin(\theta/2) \\ ie^{i\varphi}\cos(\theta/2) \\ 0 \\ 0 \end{pmatrix}, \tag{S3}$$

where $\varphi$ defines the direction of $\mathbf{p} = \hbar\mathbf{k}$ with respect the positive direction of the x-axis, $p_x/p = \cos\varphi$, and the angle $\theta$, which fixes the"helicity" direction and determines the *effective* strength of the spin-orbit coupling, is defined as $\cos\theta = 1/\sqrt{1 + (\eta p/\hbar\epsilon_-)^2}$, $\varepsilon_- = \Delta/2 = (\varepsilon_o - \varepsilon_e)/2$. For simplicity we use the notation such as $|\Psi_{1,\uparrow}\rangle$, however we recall that the spin direction $\sigma$ in the corresponding state is determined by the helicity axis given by the angle $\theta$. The Hamiltonian (S1) has the structure of two independent Rashba-like Hamiltonians. Note, however, that in the basis indicated above the spin operator $\hat{S}_x$ reads

$$\hat{S}_x = \frac{1}{2} \begin{pmatrix} 0 & \hat{\sigma}_x \\ \hat{\sigma}_x & 0 \end{pmatrix}.$$

Therefore the average value of the x-component of the spin is zero, $< \Psi_{1,\uparrow}|\hat{S}_x|\Psi_{1,\uparrow} >= 0$ (the same is true for the y-component). In contrast, the $\hat{S}_z$ spin operator is diagonal in the basis in question

$$\hat{S}_z = \frac{1}{2}\begin{pmatrix} \hat{\sigma}_z & 0 \\ 0 & \hat{\sigma}_z \end{pmatrix}.$$

Therefore the procedure for calculating the average z-component of the spin (main text) is similar to the procedure in the case of usual Rashba one-band Hamiltonian. In particular, in the limit $\varepsilon_o - \varepsilon_e \to 0$, when $\theta \to \pi/2$, we have two identical Rashba Hamiltonians with the same solutions, see, for example, Eq. (S2).

The SO Hamiltonian of our problem only mixes states belonging to different subbands and having opposite spins. For any potential scattering (either by impurities or by sample boundaries) only functions $\Psi_{1,\uparrow}$ and $\Psi_{2,\downarrow}$ are coupled. The other coupled pair $\Psi_{1,\downarrow}$ and $\Psi_{2,\uparrow}$ is totally independent of the first pair.

## II. BOUNDARY SCATTERING AMPLITUDES

From Eqs. (4), (5) of the main text we obtain for the boundary scattering amplitudes

$$F_{1,\uparrow}^{1,\uparrow} = [e^{-i\varphi_1}\sin(\theta_1/2)\sin(\theta_2/2) - e^{i\varphi_2}\cos(\theta_1/2)\cos(\theta_2/2)]/D, \tag{S4}$$

$$F_{1,\uparrow}^{2,\downarrow} = -\sin\theta_1\cos\varphi_1/D, \tag{S5}$$

$$F_{2,\downarrow}^{2,\downarrow} = -[e^{i\varphi_1}\sin(\theta_1/2)\sin(\theta_2/2) - e^{-i\varphi_2}\cos(\theta_1/2)\cos(\theta_2/2)]/D; \tag{S6}$$

$$F_{2,\downarrow}^{1,\uparrow} = -\sin\theta_2\cos\varphi_2/D, \tag{S7}$$

$$D = e^{i\varphi_2}\cos(\theta_1/2)\cos(\theta_2/2) + e^{i\varphi_1}\sin(\theta_1/2)\sin(\theta_2/2). \tag{S8}$$

From the above equations we can find the components of the unitary scattering matrix $\hat{S}$

$$S_{1,\uparrow}^{1,\uparrow} = F_{1,\uparrow}^{1,\uparrow},\ S_{2,\downarrow}^{2,\downarrow} = F_{2,\downarrow}^{2,\downarrow},\ S_{1,\uparrow}^{2,\downarrow} = S_{2,\downarrow}^{1,\uparrow} = F_{1,\uparrow}^{2,\downarrow}\sqrt{\frac{v_{x,2}}{v_{x,1}}}, \tag{S9}$$

where the group velocities in the sub-bands $i = 1, 2$ are $v_{x,i} = \partial\varepsilon_i/\partial p_x$.

The formulas for the scattering amplitudes for the case of other coupled pair of functions, $\Psi_{1,\downarrow}(\varphi_1), \Psi_{2,\uparrow}(\varphi_2)$, can be obtained from the above formulas with the help of the following replacements. First of all one needs to make the replacements $\cos(\theta_1/2) \leftrightarrows \sin(\theta_1/2)$, $\cos(\theta_2/2) \leftrightarrows \sin(\theta_2/2)$ in the expression for $D$ (S8). Then to obtain $F_{1,\downarrow}^{2,\uparrow}$ from $F_{1,\uparrow}^{2,\downarrow}$ and

$F^{1,\downarrow}_{2,\uparrow}$ from $F^{1,\uparrow}_{2,\downarrow}$ no further replacements are needed; however, to obtain $F^{1,\downarrow}_{1,\downarrow}$ from $F^{1,\uparrow}_{1,\uparrow}$ and $F^{2,\uparrow}_{2,\uparrow}$ from $F^{2,\downarrow}_{2,\downarrow}$, the replacements above should also be made in Eqs (S4) and (S6). The corresponding scattering matrix elements $S^{1,\downarrow}_{1,\downarrow}$, $S^{2,\uparrow}_{2,\uparrow}$, $S^{2,\uparrow}_{1,\downarrow} = S^{1,\downarrow}_{2,\uparrow}$ are also determined.

From Eqs. (4)-(7) of the main text we obtain

$$\langle S_z(x)\rangle = \mathrm{Re}\Bigg\{ \int \frac{dk_y}{(2\pi)^2} \frac{d\varepsilon}{\sqrt{v_{x,1} v_{x,2}}} \left[ S^{2,\uparrow}_{2,\uparrow} \cdot (S^{1,\downarrow}_{2,\uparrow})^\star \cdot \langle \Psi_{1,\downarrow}(\varphi_1)|\hat{\sigma}_z|\Psi_{2,\uparrow}(\varphi_2)\rangle + (\uparrow\leftrightarrows\downarrow)\right] \times e^{i(k_1-k_2)x}[f_1(\varepsilon,k_y) - f_2(\varepsilon,k_y)] \Bigg\}. \quad \text{(S10)}$$

Using expressions (S2)-(S9) we find

$$\langle S_z(x)\rangle = -\int \frac{dk_y}{(2\pi)^2} \frac{d\varepsilon}{\sqrt{v_1 v_2}} \left[ k_y \frac{\sqrt{\sin\theta_1 \sin\theta_2}(p_1^{-1}\sin\theta_1 + p_2^{-1}\sin\theta_2)}{\cos^2[(\theta_1-\theta_2)/2] - \sin\theta_1\sin\theta_2\sin^2[(\varphi_1-\varphi_2)/2]} \right] \times \sin[(p_1\cos\varphi_1 - p_2\cos\varphi_2)x/\hbar][f_1(\varepsilon,k_y) - f_2(\varepsilon,k_y)]. \quad \text{(S11)}$$

The angles $\theta_1, \theta_2$ are defined via $\cos\theta_{1,2} = 1/\sqrt{1+(\eta p_{1,2}/\hbar\varepsilon_-)^2}$.

## III. DISTRIBUTION FUNCTIONS DUE TO IMPURITY SCATTERING IN THE 2DEG ("BULK")

We determine here the expressions for the non-equilibrium distribution functions entering Eq. (8) of the main text. We recall that $f_i(\varepsilon, k_y)$ is the distribution function of the electron state in the sub-band $i = 1,2$ for a given energy and given wave vector $k_y$ along the boundary. They are formed by the impurity scattering in the 2D bulk of a sample in the presence of electric field. We will calculate them in the Born approximation (i.e. the lowest order perturbation theory) in the impurity scattering amplitudes following the procedure developed in [2].

In general, in the presence of spin-orbit coupling the electron states are described by the spin-density matrix. In the helicity basis which diagonalizes the Hamiltonian this matrix contains both diagonal and non-diagonal elements. The diagonal elements (i.e., the distribution functions) describe the populations of the states with a given helicity and the non-diagonal elements describe the coherence between the states of different helicities. For the two-subband problem we consider here, the states within the bands 1 and 2 (for a given

momentum) correspond to different helicities. Since we consider the quasi-ballistic case (i.e. the energy separation between two sub-bands $\tilde{\Delta} = \sqrt{\Delta^2 + 4\eta^2 k_F^2}$ is much larger than $\hbar/\tau_{tr}$), the non-diagonal elements of the spin-density matrix are small as compared to the diagonal ones: $f_{12} \simeq f_{11}/(\tilde{\Delta}\tau_{tr}) \ll f_{11}$. Thus in calculating the diagonal elements $f_{11} \equiv f_1, f_{22} \equiv f_2$ (these functions do not depend on the "spin" direction, e.g., $f_{1,\uparrow} = f_{1,\downarrow} = f_1$ ) we can neglect in the collision integral all the non-diagonal elements and deal with the standard Boltzmann equations for the distribution functions [2].

We consider a smooth impurity potential (i.e. the scattering of the small-angle type) and assume the conditions $k_F^{-1} \ll d \ll L_s$, where $d$ is the correlation radius of the impurity potential in the bulk of the structure. In addition, we consider the case when $p_1 - p_2 \ll p_F$, see Fig.1, which means that the energy difference between two sub-bands is much smaller than the Fermi energy (as in the experiment).

The quantity we need to calculate is $f_1(\varepsilon_F, k_y) - f_2(\varepsilon_F, k_y)$, see Eq. (8) of the main text and Fig. 1. Taking into account that the distribution function in the presence of the electric field directed along the y-axis has the form $f(\mathbf{p}) = f(p)\hbar k_y/p$ (i.e., it is proportional to the cosine of angle between the momentum and the electric field vector [2]), we obtain

$$f_1(\varepsilon_F, k_y) - f_2(\varepsilon_F, k_y) = \left(\frac{f_1(p_1)}{p_1} - \frac{f_2(p_2)}{p_2}\right)\hbar k_y. \tag{S12}$$

Then for the scalar functions $f_1(p_1)$, $f_2(p_2)$ we have the system of kinetic equations

$$a^{-1}\frac{eEp_1}{m}\frac{\partial f_0}{\partial \varepsilon} = -f_1(p_1)\frac{a}{\tau_{tr}(p_1)} - (f_1(p_1) - f_2(p_2))\frac{b\sin^2\theta}{2\tau_{tr}(p_F)}, \tag{S13}$$

$$b^{-1}\frac{eEp_2}{m}\frac{\partial f_0}{\partial \varepsilon} = (f_1(p_1) - f_2(p_2))\frac{a\sin^2\theta}{2\tau_{tr}(p_F)} - f_2(p_2)\frac{b}{\tau_{tr}(p_2)}. \tag{S14}$$

These equations are obtained in the standard way (Fermi's Golden rule) by calculating the matrix elements of an impurity potential between the states described by the functions (S2), (S3). In calculating these matrix elements we have used that scattering is of the small-angle type and that $p_1 - p_2 \ll p_F$. The quantities entering Eqs. (S13) and (S14) have the following meaning

$$\frac{1}{\tau_{tr}(p)} = m\int_0^\infty (\frac{d\vartheta}{\pi})\frac{\vartheta^2}{2}W(p\vartheta) \tag{S15}$$

is the inverse transport scattering time corresponding to a small-angle scattering case (we have extended the upper limit $\pi$ up to $\infty$) [3], $W(p\vartheta) = n_i|U(p\vartheta)|^2/2\hbar^3$, $n_i$ is the 2D impurity density and $U(p\vartheta)$ is the Fourier component of impurity potential corresponding

to the momentum transfer $2p|\sin(\vartheta/2)| \approx p\vartheta$, $\vartheta$ is the scattering angle (do not confuse with the angle $\theta$!). The factors

$$a^{-1} = (1 - \frac{2m\eta^2}{\hbar^2\Delta}\cos\theta); \;\; b^{-1} = (1 + \frac{2m\eta^2}{\hbar^2\Delta}\cos\theta) \tag{S16}$$

with $\cos\theta = 1/\sqrt{1+(2\eta k_F/\Delta)^2}$ determine the group velocities at the corresponding momenta in the subbands 1 and 2: $\partial\varepsilon_1/\partial p_1 = a^{-1}p_1/m$, $\partial\varepsilon_2/\partial p_2 = b^{-1}p_2/m$. In the approximation we consider here $ab = 1$ (higher order terms should be neglected). Note that the inter-subband terms in Eqs. (S13) and (S14), which are proportional to $\sin^2\theta$, contain $\tau_{tr}(p_F)$ at the Fermi momentum, i.e., in calculating these terms we have neglected the energy separation between the sub-bands. Strictly speaking this is true when $(p_1-p_2)d/\hbar \ll 1$. We assume that $d \ll L_s$, however, since $p_1 - p_2 = \hbar\sqrt{1/L_s^2 + 1/L_\Delta^2}$ the condition $(p_1 - p_2)d/\hbar \ll 1$ is violated for small enough $L_\Delta$ when $L_\Delta \ll L_s$. Since the terms in question (inter-subband ones) contain also $\sin^2\theta$ which in the limit considered is $\sin^2\theta \approx L_\Delta^2/L_s^2 \ll 1$, they will be neglected in this limit anyway, while calculating $f_1(\varepsilon_F, k_y) - f_2(\varepsilon_F, k_y)$ (see below). Therefore the approximation in question is valid.

It can be checked that Eqs. (S13) and (S14) coincide in the limit $\Delta \to 0$ with the corresponding equations for the single-band usual Rashba model (and the small-angle scattering case). On the other hand, with increasing the gap value the $\sin^2\theta$ factor, which determines the probability of spin-flip and enters the inter-subband transition rate [see Eqs. (S13) and (S14)], decreases. Thus eventually the inter-subbands terms can be neglected. This leads to the usual distribution functions (Eq. (11) of the main text), lack of the specific cancellation inherent for the single-band Rashba model, and recovering of the first order effect with respect to small splitting $p_1 - p_2 \ll p_F$ for the edge spin density.

From Eqs. (S13) and (S14) and within the approximations outlined above we obtain

$$f_1(\varepsilon_F, k_y) - f_2(\varepsilon_F, k_y) = -\frac{eE\hbar k_y}{m}\frac{\partial f_0}{\partial\varepsilon}\frac{\tau_{tr}(p_F)}{(1+\sin^2\theta)} \times \left[\left(\frac{b^2}{\tau_{tr}(p_2)} - \frac{a^2}{\tau_{tr}(p_1)}\right)\tau_{tr}(p_F) - \sin^2\theta\frac{(p_1-p_2)}{p_F}\right], \tag{S17}$$

where $a^2 = 1 + (4m\eta^2\cos\theta/\hbar^2\Delta)$ and $b^2 = 1 - (4m\eta^2\cos\theta/\hbar^2\Delta)$. Expanding $(\tau_{tr}(p_1) - \tau_{tr}(p_2))/\tau_{tr} \approx 3(p_1 - p_2)/p_F$ (with the use of the small-angle scattering condition), we finally

obtain

$$f_1(\varepsilon_F,k_y)-f_2(\varepsilon_F,k_y)=-\frac{\hbar^2 k_y k_E}{m k_F L_s}\frac{\partial f_0}{\partial\varepsilon}\frac{3\cos^2\theta}{\sin\theta(1+\sin^2\theta)} \tag{S18}$$

To obtaint the above result we have used $p_1-p_2=\hbar/\Lambda$, with $\Lambda=L_\Delta L_s/\sqrt{L_\Delta^2+L_s^2}$, and denoted $k_E=eE\tau_{tr}/\hbar$. Note that $\cos\theta=L_s/\sqrt{L_s^2+L_\Delta^2}$.

---


[1] E. Bernardes, J. Schliemann, M. Lee, J. C. Egues, and D. Loss, Phys. Rev. Lett. **99**, 076603 (2007).

[2] A. Khaetskii, Phys. Rev. B **73**, 115323 (2006).


[3] Note that introducing in Eq. (S15) the new variable $p\vartheta$, we obtain the following momentum dependence of the transport scattering time in a small-angle scattering case, $\tau_{tr}(p)=Ap^3$, where $A$ is some constant.
